# Supplementary material for: A Coordinate-wise Optimization Algorithm for Sparse Inverse Covariance Selection
Source: arXiv:1711.07038 source file (2018-04-04)
Supplement: Supplementary file 1 [file appendix.tex]

\clearpage
{\LARGE
\bbb{Appendix}
}
%\appendix
%\renewcommand\thesection{\appendixname~\Roman{section}}
%\renewcommand\theequation{\Alph{section}.\arabic{equation}}
%\setcounter{equation}{0}
%\setcounter{theorem}{0}
